# Supplementary material for: Density Classification with Non-Unitary Quantum Cellular Automata
Source: arXiv:2404.05461 source file (2025-01-20)
Supplement: Supplementary file 1 [file excluded_appendices.tex]

\ew{The following appendices are just notes:}

\subsection{Unital property of the Dephasing QCA}

The Dephasing QCA is unital with $\hat{\mathcal{L}}^\tx{(Dephasing)}\qty[\hat{\mathds{1}}]=0$.
 
This is derived by noting that the Hamiltonian commutes with the identity operator, $\qty[\hat{H},\hat{\mathds{1}}]=0$, and that $\hat{L}_1+\hat{L}_2+\hat{L}_3+\hat{L}_4=\hat{\mathds{1}}$ because $\hat{L}_1+\hat{L}_4=\hat{P}_0\otimes\hat{P}_0+\hat{P}_1\otimes\hat{P}_1=\hat{\mathds{1}}-\hat{P}_0\otimes\hat{P}_1-\hat{P}_1\otimes\hat{P}_0$ and $\hat{L}_2+\hat{L}_3=\hat{P}_0\otimes\hat{P}_1+\hat{P}_1\otimes\hat{P}_0$, such that the dissipator vanishes as its summands $\sum_{k=1}^4\qty(\hat{L}_{k_j}\otimes\hat{L}_{k_j})=\hat{\mathds{1}}=\frac{1}{2}\sum_{k=1}^4\qty(\hat{L}_{k_j}\otimes\hat{\mathds{1}} + \hat{\mathds{1}}\otimes\hat{L}_{k_j})$ cancel each other out.

\subsection{Dephasing QCA}

Next, the in Sec.~\ref{sec:dephasing} defined Dephasing QCA is investigated. It can be shown that $\hat{\mathcal{L}}^\tx{(Dephasing)}[\hat\rho]$ conserves the number density of $\hat\rho$ with $\frac{\tx d}{\tx dt}\expval{\hat{S}_z(t)} = 0$, see proof in App.~\ref{app:SzDephasing}.
The corresponding steady state is the sum of all pure states with the same global number density:
\ba
    \hat\rho_{\tx{ss}_m}^\tx{(Dephasing)}
    =
    \frac{1}{\mqty(N\\m)}
    \sum_{\pi \ \tx{permutations}} \dyad*{\pi(\underbrace{0...0}_{N-m}\underbrace{1...1}_{m})},
\ea
where $\mqty(N\\m)=\frac{m!(N-m)!}{N!}$ and $\frac{m}{N}$ is the number density the initial state. The proof is outlined with more examples in App.~\ref{app:dcdephasing}, but follows directly from the unital property of the Lindbladian, $\hat{\mathcal{L}}^\tx{(Dephasing)}\qty[\hat{\mathds{1}}]=0$, its translational invariance, and the conservation of $\hat{S}_z=\frac{1}{2}\sum_j \hat Z_j$ $\forall\,\Omega$; see derivation in App.~\ref{app:SzDephasing}.
Hence, there are $(N+1)$ steady states for every system size $N\in\mathbb{N_+} \ \forall\ \Omega,\gamma\in\mathbb{R}$. For instance for $N=3$, these are for the set of initial number densities $\frac{m}{N}\in\big\{0;\frac{1}{3};\frac{2}{3};1\big\}$:
$\Big\{\hat\rho_{\tx{ss}_m}^\tx{(Dephasing)}\Big\}_{m=0}^3=\big\{\dyad{000};\frac{1}{3}(\dyad{001} + \dyad{010} + \dyad{100});\frac{1}{3}(\dyad{011} + \dyad{101} + \dyad{110});\dyad{111}\big\}$.

\section{Steady states of the Dephasing QCA}
In this section, the steady states of the Dephasing QCA are derived, see definition in Sec.~\ref{sec:dephasing}.
The proof follows from the three following properties of the Lindbladian:
\begin{itemize}
    \item It is unital with $\hat{\mathcal{L}}^\tx{(Dephasing)}\qty[\hat{\mathds{1}}]=0$ \footnote{The proof follows directly from Eqs.~\eqref{eq:LioDephasing0011local0} and \eqref{eq:LioDephasing010} given $\hat{\mathds{1}}_{j,j+1}=P_{0_j}P_{0_{j+1}}+P_{1_j}P_{1_{j+1}}+P_{0_j}P_{1_{j+1}}+P_{1_j}P_{0_{j+1}}$}.
    \item It conserves the global number density with $\qty(\hat{\mathcal{L}}^\tx{(Dephasing)})^{\!\dagger} \qty[\hat{S}_z]=0$, as shown in App.~\ref{app:SzDephasing}.
    \item It is translationally invariant.
\end{itemize}
The last point shows that because if $\ket{\hat\rho_\tx{ss}}$ with $\hat{\mathbb{L}}\ket{\hat\rho_\tx{ss}}=0$ is a vectorized steady state of a system defined by a translationally invariant Lindbladian $\hat{\mathbb{L}}$, then $\hat{T}\hat\rho_\tx{ss}\hat{T}^\dagger \rightarrow \hat{T}\otimes \hat{T}^* \ket{\hat\rho_\tx{ss}}$, with translation operator $\hat{T}$, must also be a steady state of the same system as
\ba
    \hat{\mathbb{L}} \qty(\hat{T}\otimes\hat{T}^*) \ket{\hat\rho_\tx{ss}}
    &= \qty(\hat{T}\otimes\hat{T}^*) \underbrace{\qty(\hat{T} \otimes \hat{T}^*)^{\!\dagger} \; \hat{\mathbb{L}} \; \qty(\hat{T}\otimes\hat{T}^*)}_{=\hat{\mathbb{L}}} \ket{\hat\rho_\tx{ss}} \nn\\
    &= \qty(\hat{T}\otimes\hat{T}^*) \,\hat{\mathbb{L}} \,\ket{\hat\rho_\tx{ss}} \nn\\
    &= 0,
\ea
such that any single site translation of a steady state is also a steady state.

Hence, given the translational invariance and the preservation of $\hat{\mathds{1}}$ and $\hat{S}_z$, the projection of the identity operator onto the $\hat{S}_z$ eigenspace $\ev{\hat{S}_z}=-\frac{N}{2}-m$, $\hat{P}_{\ev{\hat{S}_z}=-\frac{N}{2}-m} \hat{\mathds{1}} \hat{P}_{\ev{\hat{S}_z}=-\frac{N}{2}-m}$, represents the set of steady states of the system, which is the sum of all states with the same number density:
\ew{TBC: coherence terms}
\ba
    \hat\rho_\tx{ss}^\tx{(Dephasing)}
    =
    \frac{1}{\mqty(N\\m)}%\frac{N!}{m!(N-m)!}
    \sum_{\pi \ \tx{permutations}} \dyad*{\pi(\underbrace{0...0}_{N-m}\underbrace{1...1}_{m})},
\ea
where $\mqty(N\\m)=\frac{m!(N-m)!}{N!}$, $N$ represents the total number of sites and $m$ is the number of ones of the initial state.
\iffalse
\gkb{Don't really need to give the explicit states for $N=4,5$, the reader can figure it out. You could include it for the thesis.}
The set of steady states $\hat\rho_\tx{ss}^\tx{(Dephasing)} = \{ \hat\rho_1,...,\hat\rho_{_{N+1}} \}$ is for example for $N=4$ $\forall\ \Omega,\gamma$:
\bs
\ba
    \hat\rho_1 &= \dyad{0000}, \\
    \hat\rho_2 &= \dyad{1111}, \\
    \hat\rho_3 &= \frac{1}{4}(\dyad{0001} + \dyad{0010} + \dyad{0100} + \dyad{1000}), \\
    \hat\rho_4 &= \frac{1}{4}(\dyad{0111} + \dyad{1011} + \dyad{1101} + \dyad{1110}), \\
    \hat\rho_5 &= \frac{1}{6}
    (\dyad{0011} 
    + \dyad{0101} 
    + \dyad{0110}
    + \dyad{1001} 
    + \dyad{1010} 
    + \dyad{1100}),
\ea\es
and for $N=5$:
\bs
\ba
    \hat\rho_1 &= \dyad{00000}, \\
    \hat\rho_2 &= \dyad{11111}, \\
    \hat\rho_3 &= \frac{1}{5}
    (\dyad{00001} 
    + \dyad{00010} 
    + \dyad{00100}
    + \dyad{01000} 
    + \dyad{10000}), \\
    \hat\rho_4 &= \frac{1}{5}
    (\dyad{01111}
    + \dyad{10111} 
    + \dyad{11011}
    + \dyad{11101} 
    + \dyad{11110}),
    \\
    \hat\rho_5 &= \frac{1}{10}
    (\dyad{00011} 
    + \dyad{00101} 
    + \dyad{00110}
    + \dyad{01001} 
    + \dyad{01010} \nn\\&\qquad\qquad 
    + \dyad{01100}
    + \dyad{10001} 
    + \dyad{10010} 
    + \dyad{10100} 
    + \dyad{11000}), \\
    \hat\rho_6 &= \frac{1}{10}
    (\dyad{00111} 
    + \dyad{01011} 
    + \dyad{01101}
    + \dyad{01110} 
    + \dyad{10011} \nn\\&\qquad\qquad  
    + \dyad{10101}
    + \dyad{10110} 
    + \dyad{11001} 
    + \dyad{11010} 
    + \dyad{11100}).
\ea\es 
\fi

To provide a few exemplary proofs for clarification, it is for instance straightforward to show the all zero and the all one states are steady states, given
\bs
\ba
    \hat{\mathcal{L}}^\tx{(Dephasing)}\qty[\dyad{0...0}]&=0, \\
    \hat{\mathcal{L}}^\tx{(Dephasing)}\qty[\dyad{1...1}]&=0.
\ea
\label{eq:LioDephasing0011}\es
Analogously to the derivation of the steady states of the \Fuks\ QCA in App.~\ref{app:steadystatesfuks}, it suffices to inspect the two-cell neighborhoods on which the Lindbladian acts on non-trivially due to the translational invariance of the operator: 
\bs
\ba
    \hat{\mathcal{L}}^\tx{(Dephasing)}\qty[\dyad{0...0}]
    &=\sum_{j} \hat{\mathcal{L}}_{j,j+1}^\tx{(Dephasing)}\qty[\dyad{00}_{j,j+1}], \\
    \hat{\mathcal{L}}^\tx{(Dephasing)}\qty[\dyad{1...1}]
    &=\sum_{j} \hat{\mathcal{L}}_{j,j+1}^\tx{(Dephasing)}\qty[\dyad{11}_{j,j+1}].
\ea
\label{eq:LioDephasing0011local}\es
Considering the local Lindbladian acting on the $\dyad{00}=\hat{P}_0\hat{P}_0$ state at the two neighboring sites ${j,j+1}$, one can show that, firstly, the Hamiltonian term is vanishing $\forall\,\Omega$ with
\ba
    \qty[\hat{X}_j\hat{X}_{j+1}+\hat{Y}_j\hat{Y}_{j+1} \ , \hat{P}_{0_j} \hat{P}_{0_{j+1}}]
    &=
    \qty[\hat{X}_j\hat{X}_{j+1}\ , \hat{P}_{0_j} \hat{P}_{0_{j+1}}] 
    +
    \qty[\hat{Y}_j\hat{Y}_{j+1} \ , \hat{P}_{0_j} \hat{P}_{0_{j+1}}] \nn\\
    &=
    \qty(\hat\sigma^+_j \hat\sigma^+_{j+1}
    -\hat\sigma^-_j \hat\sigma^-_{j+1})
    +\qty(-\hat\sigma^+_j \hat\sigma^+_{j+1}
    +\hat\sigma^-_j \hat\sigma^-_{j+1})
    = 0,
\ea
and, secondly, the dissipator is zero $\forall\,\gamma$, because
\ba
    \sum_{k=1}^4 &\qty(
    \hat{L}_{k_{j,j+1}}\qty(\hat{P}_{0_j}\hat{P}_{0_{j+1}}) \hat{L}_{k_{j,j+1}}^\dagger 
    -\frac{1}{2}
    \qty(\qty(\hat{P}_{0_j}\hat{P}_{0_{j+1}}) \hat{L}_{k_{j,j+1}}^\dagger \hat{L}_{k_{j,j+1}} + \hat{L}_{k_{j,j+1}}^\dagger \hat{L}_{k_{j,j+1}} \qty(\hat{P}_{0_j}\hat{P}_{0_{j+1}}))) \nn\\
    &=
    \hat{L}_{1_{j,j+1}} \qty(\hat{P}_{0_j}\hat{P}_{0_{j+1}}) \hat{L}_{1_{j,j+1}}^\dagger 
    -\frac{1}{2}
    \qty(\qty(\hat{P}_{0_j}\hat{P}_{0_{j+1}}) \hat{L}_{1_{j,j+1}}^\dagger \hat{L}_{1_{j,j+1}} + \hat{L}_{1_{j,j+1}}^\dagger \hat{L}_{1_{j,j+1}} \qty(\hat{P}_{0_j}\hat{P}_{0_{j+1}})) \nn\\
    &=
    \hat{P}_{0_j}\hat{P}_{0_{j+1}}
    -\frac{1}{2}
    \qty(\hat{P}_{0_j}\hat{P}_{0_{j+1}} + \hat{P}_{0_j}\hat{P}_{0_{j+1}})
    = 0.
\ea
This leads to
\bs
\ba
    \hat{\mathcal{L}}_{j,j+1}^\tx{(Dephasing)}\qty[\hat{P}_{0_j} \hat{P}_{0_{j+1}}] &=0, \\
    \hat{\mathcal{L}}_{j,j+1}^\tx{(Dephasing)}\qty[\hat{P}_{1_j} \hat{P}_{1_{j+1}}] &=0,
\ea\label{eq:LioDephasing0011local0}\es
where the derivation of $\hat{\mathcal{L}}_{j,j+1}\qty[\hat{P}_{1_j} \hat{P}_{1_{j+1}}]=0$ follows from the $\hat{\mathbb{Z}}_2$-symmetry of the Hamiltonian and jump operators. According to Eqs.~\eqref{eq:LioDephasing0011local} and \eqref{eq:LioDephasing0011local0}, Eq.~\eqref{eq:LioDephasing0011} has thus been proved.

Next, the states $\dyad{0...010...0}$ and $\dyad{1...101...1}$, where one site is in a different state than the rest, are shown to decay and not be steady states, as
\bs
\ba
    \hat{\mathcal{L}}^\tx{(Dephasing)}\qty[\dyad{0...0_{j-1}1_j0_{j+1}...0}]
    &\neq0, \\
    \hat{\mathcal{L}}^\tx{(Dephasing)}\qty[\dyad{1...1_{j-1}0_j1_{j+1}...1}]
    &\neq0.
\ea
\label{eq:LioDephasing010}\es
Because all terms acting on two neighboring zero or one states are zero, $\hat{\mathcal{L}}_{j,j+1}^\tx{(Dephasing)}\qty[\dyad{00}_{j,j+1}]=0=\hat{\mathcal{L}}_{j,j+1}^\tx{(Dephasing)}\qty[\dyad{11}_{j,j+1}]$, see Eq.~\eqref{eq:LioDephasing0011local0}, Eq.~\eqref{eq:LioDephasing010} yields:
\bs
\ba
    \hat{\mathcal{L}}^\tx{(Dephasing)}\qty[\dyad{0...0_{j-1}1_j0_{j+1}...0}]
    &=\hat{\mathcal{L}}_{j-1,j}^\tx{(Dephasing)}\qty[\dyad{01}_{j-1,j}]+\hat{\mathcal{L}}_{j,j+1}^\tx{(Dephasing)}\qty[\dyad{10}_{j,j+1}],\\
    \hat{\mathcal{L}}^\tx{(Dephasing)}\qty[\dyad{1...1_{j-1}0_j1_{j+1}...1}]
    &=\hat{\mathcal{L}}_{j-1,j}^\tx{(Dephasing)}\qty[\dyad{10}_{j-1,j}]+\hat{\mathcal{L}}_{j,j+1}^\tx{(Dephasing)}\qty[\dyad{01}_{j,j+1}].
\ea
\label{eq:LioDephasing010local}\es
 due to the translational invariance of the Lindbladian.
By reflection symmetry around two neighboring sites $j$ and $j+1$ of the Hamiltonian and the jump operators, one can find that
\ba
    &\hat{\mathcal{L}}_{j,j+1}^\tx{(Dephasing)}\qty[\hat{P}_{0_j} \hat{P}_{1_{j+1}}]
    =-\hat{\mathcal{L}}_{j,j+1}^\tx{(Dephasing)}\qty[\hat{P}_{1_j} \hat{P}_{0_{j+1}}],
    \label{eq:LioDephasing010minus}
\ea
where
\ba
    &\hat{\mathcal{L}}_{j,j+1}^\tx{(Dephasing)}\qty[\hat{P}_{0_j} \hat{P}_{1_{j+1}}]
    =
    -2i\,\Omega\,\qty(\hat\sigma^+_j \hat\sigma^-_{j+1}
    -\hat\sigma^-_j \hat\sigma^+_{j+1})
    +\frac{\gamma}{2}
    \qty(-\hat{P}_{0_j}\hat{P}_{1_{j+1}}
    +\hat{P}_{1_j}\hat{P}_{0_{j+1}}),
    \label{eq:LioDephasing010localresult}
\ea
as the Hamiltonian term leads to 
\ba
    \qty[\hat{X}_j\hat{X}_{j+1}+\hat{Y}_j\hat{Y}_{j+1} \ , \hat{P}_{0_j} \hat{P}_{1_{j+1}}]
    &=
    \qty[\hat{X}_j\hat{X}_{j+1}\ , \hat{P}_{0_j} \hat{P}_{1_{j+1}}] 
    +
    \qty[\hat{Y}_j\hat{Y}_{j+1} \ , \hat{P}_{0_j} \hat{P}_{1_{j+1}}] \nn\\
    &=
    \qty(\hat\sigma^+_j \hat\sigma^-_{j+1}
    -\hat\sigma^-_j \hat\sigma^+_{j+1})
    +\qty(\hat\sigma^+_j \hat\sigma^-_{j+1}
    -\hat\sigma^-_j \hat\sigma^+_{j+1}) \nn\\
    &=
    2\qty(\hat\sigma^+_j \hat\sigma^-_{j+1}
    -\hat\sigma^-_j \hat\sigma^+_{j+1}),
\ea
and the dissipator is
\ba
    \sum_{k=1}^4 &\underbrace{\qty(
    \hat{L}_{k_{j,j+1}}\qty(\hat{P}_{0_j}\hat{P}_{1_{j+1}}) \hat{L}_{k_{j,j+1}}^\dagger 
    -\frac{1}{2}
    \qty(\qty(\hat{P}_{0_j}\hat{P}_{1_{j+1}}) \hat{L}_{k_{j,j+1}}^\dagger \hat{L}_{k_{j,j+1}} + \hat{L}_{k_{j,j+1}}^\dagger \hat{L}_{k_{j,j+1}} \qty(\hat{P}_{0_j}\hat{P}_{1_{j+1}})))
    }_{=\begin{cases}0 &\forall\,k=1,4 \\\frac{1}{4}
    \qty(-\hat{P}_{0_j}\hat{P}_{1_{j+1}}
    +\hat{P}_{1_j}\hat{P}_{0_{j+1}}) &\forall\,k=2,3 \end{cases}} \nn\\
    &=
    \frac{1}{2}
    \qty(-\hat{P}_{0_j}\hat{P}_{1_{j+1}}
    +\hat{P}_{1_j}\hat{P}_{0_{j+1}}).
\ea
Hence, 
\bs
\ba
    \hat{\mathcal{L}}_{j-1,j}^\tx{(Dephasing)}\qty[\dyad{01}_{j-1,j}]+\hat{\mathcal{L}}_{j,j+1}^\tx{(Dephasing)}\qty[\dyad{10}_{j,j+1}]&\neq0,\\
    \hat{\mathcal{L}}_{j-1,j}^\tx{(Dephasing)}\qty[\dyad{10}_{j-1,j}]+\hat{\mathcal{L}}_{j,j+1}^\tx{(Dephasing)}\qty[\dyad{01}_{j,j+1}]&\neq0,
\ea\es
because the Lindbladian acts on two different two-cell neighborhoods; such that with Eq.~\eqref{eq:LioDephasing010local}, Eq.~\eqref{eq:LioDephasing010} has been proved.

Furthermore, considering two (or more) neighboring states that are orthogonal to all other states, one can similarly see with Eqs.~\eqref{eq:LioDephasing010local} to \eqref{eq:LioDephasing010localresult}, that:
\bs
\ba
    &\hat{\mathcal{L}}^\tx{(Dephasing)}\qty[\dyad{0...0_{j-1}1_j1_{j+1}0_{j+2}...0}]\nn\\
    &\qquad=\hat{\mathcal{L}}_{j-1,j}^\tx{(Dephasing)}\qty[\dyad{01}_{j-1,j}]+\hat{\mathcal{L}}_{j+1,j+2}^\tx{(Dephasing)}\qty[\dyad{10}_{j+1,j+2}]\neq0,
\ea
and
\ba
    &\hat{\mathcal{L}}^\tx{(Dephasing)}\qty[\dyad{1...1_{j-1}0_j0_{j+1}1_{j+2}...1}]\nn\\
    &\qquad=\hat{\mathcal{L}}_{j-1,j}^\tx{(Dephasing)}\qty[\dyad{10}_{j-1,j}]+\hat{\mathcal{L}}_{j+1,j+2}^\tx{(Dephasing)}\qty[\dyad{01}_{j+1,j+2}]\neq0.
\ea
\label{eq:LioDephasing0110}\es

Additionally, off-diagonal coherence terms are decaying too, because
\bs
\ba
    \hat{\mathcal{L}}^\tx{(Dephasing)}\qty[\dyad{\vec{x}_L 1_j \vec{x}_R}{\vec{x}_L 0_j \vec{x}_R}]
    &\neq0,\\
    \hat{\mathcal{L}}^\tx{(Dephasing)}\qty[\dyad{\vec{x}_L 0_j \vec{x}_R}{\vec{x}_L 1_j \vec{x}_R}]
    &\neq0,
\ea\es
$\forall \; x_L=[x_1...x_{j-1}]$ and $x_R=[x_{j+1}...x_{N}]$ with $x_j\in\{0,1\}$;
e.g.:
\ba
    \hat{\mathcal{L}}^\tx{(Dephasing)}\qty[\dyad{0...0}{0...0_{j-1}1_j0_{j+1}...0}]
    &=
    \hat{\mathcal{L}}_{j-1,j}^\tx{(Dephasing)}
    \qty[\dyad{00}{01}_{j-1,j}]
    +
    \hat{\mathcal{L}}_{j,j+1}^\tx{(Dephasing)}
    \qty[\dyad{00}{10}_{j,j+1}] \nn\\
    &=
    \qty(2i\Omega \dyad{00}{10}_{j-1,j} -\gamma\dyad{00}{01}_{j-1,j})
    +
    \qty(2i\Omega \dyad{00}{01}_{j,j+1} -\gamma\dyad{00}{10}_{j,j+1}) \nn\\
    &\neq0,
\ea
and analogously for the corresponding bit-flipped state due to the $\hat{\mathbb{Z}}_2$-symmetry of the Lindbladian.

However, the (normalized) sum of all states with the same number density can be shown to be a steady state. These are for example for a three-cell system (that exhibit a non-zero and non-one number density):
\bs
\ba
    \frac{1}{3}(\dyad{001} + \dyad{010} + \dyad{100}), \\
    \frac{1}{3}(\dyad{011} + \dyad{101} + \dyad{110}),
\ea
\label{eq:LioDephasing001}\es
whose Lindblad evolution can be written in terms of local two-cell neighborhoods according to Eq.~\eqref{eq:LioDephasing010local}:
\bs
\ba
    \hat{\mathcal{L}}^\tx{(Dephasing)}
    \qty[\frac{1}{3}(\dyad{001} + \dyad{010} + \dyad{100})_{1,2,3}]
    &=
    \hat{\mathcal{L}}_{2,3}^\tx{(Dephasing)}\qty[\dyad{01}_{2,3}]
    +\hat{\mathcal{L}}_{3,1}^\tx{(Dephasing)}\qty[\dyad{10}_{3,1}]
    \nn\\
    &\quad+\hat{\mathcal{L}}_{1,2}^\tx{(Dephasing)}\qty[\dyad{01}_{1,2}]+\hat{\mathcal{L}}_{2,3}^\tx{(Dephasing)}\qty[\dyad{10}_{2,3}]\nn\\
    &\quad+\hat{\mathcal{L}}_{1,2}^\tx{(Dephasing)}\qty[\dyad{10}_{1,2}]+\hat{\mathcal{L}}_{3,1}^\tx{(Dephasing)}\qty[\dyad{01}_{3,1}]\nn\\
    &=0,
\\
    \hat{\mathcal{L}}^\tx{(Dephasing)}
    \qty[\frac{1}{3}(\dyad{011} + \dyad{101} + \dyad{110})_{1,2,3}]
    &=
    \hat{\mathcal{L}}_{1,2}^\tx{(Dephasing)}\qty[\dyad{01}_{1,2}]
    +\hat{\mathcal{L}}_{3,1}^\tx{(Dephasing)}\qty[\dyad{10}_{3,1}]\nn\\
    &\quad+\hat{\mathcal{L}}_{1,2}^\tx{(Dephasing)}\qty[\dyad{10}_{1,2}]+\hat{\mathcal{L}}_{2,3}^\tx{(Dephasing)}\qty[\dyad{01}_{2,3}]\nn\\
    &\quad+\hat{\mathcal{L}}_{2,3}^\tx{(Dephasing)}\qty[\dyad{10}_{2,3}]+\hat{\mathcal{L}}_{3,1}^\tx{(Dephasing)}\qty[\dyad{01}_{3,1}]\nn\\
    &=0,
\ea
\label{eq:LioDephasing001local}\es
where all local Lindbladians acting on different states at the same two lattice sites, i.e.~$\dyad{01}_{j,j+1}$ and $\dyad{10}_{j,j+1}$, cancel each other out according to Eq.~\eqref{eq:LioDephasing010minus}.

\section{The Dephasing Lindbladian in matrix form}

\ba
    \hat{\mathbb{L}}^\tx{(Dephasing)}(\Omega,\gamma) =
    \mqty(
            M_1&0&0&0\\
            0&M_2&M_3&0\\
            0&M_3&M_2&0\\
            0&0&0&M_4
    )
\ea
with
\ba
    M_1&=\mqty(
            0&0&0&0\\
            0&-\gamma&2i\Omega&0\\
            0&2i\Omega&-\gamma&0\\
            0&0&0&-\gamma
    ), \
    &&M_2=\mqty(
        -\gamma&0&0&0\\
        0&-\gamma/2&2i\Omega&0\\
        0&2i\Omega&-\gamma/2&0\\
        0&0&0&-\gamma\\
    ), \nn\\
    M_3&=\mqty(
        -2i\Omega&0&0&0\\
        0&-2i\Omega&\gamma/2&0\\
        0&\gamma/2&-2i\Omega&0\\
        0&0&0&-2i\Omega\\
    ), \
    &&M_4=\mqty(
            -\gamma&0&0&0\\
            0&-\gamma&2i\Omega&0\\
            0&2i\Omega&-\gamma&0\\
            0&0&0&0
    ).
\ea

\section{The Dephasing Lindbladian in terms of $\hat{Z}$ and $\hat{S}^\pm$}
In the following, the Dephasing Linbladian is re-written as a function of $\hat{Z}$ and $\hat{S}^\pm=\frac{1}{2}\qty(\hat{X}\pm i\hat{Y})$. With the Hamiltonian
\ba
    \hat{H}=2\,\Omega \sum_{j} \hat{S}^+_j \hat{S}^-_{j+1}  + \hat{S}^-_j \hat{S}^+_{j+1},
\ea
and the jump operators
\ba
\begin{split}
\hat{L}_{1_{j,j+1}} &=\frac{1}{4}\qty(\mathds{\hat{1}}_j+\hat{Z}_j) \qty(\mathds{\hat{1}}_{j,j+1}+\hat{Z}_{j,j+1}), \\
\hat{L}_{2_{j,j+1}} &=\frac{1}{8}\qty(\mathds{\hat{1}}_j+\hat{Z}_j) \qty(\mathds{\hat{1}}_{j,j+1}-\hat{Z}_{j,j+1})+ \frac{1}{2}\hat{S}^+_j \hat{S}^-_{j+1} + \frac{1}{2}\hat{S}^-_j \hat{S}^+_{j+1} 
+ \frac{1}{8}\qty(\mathds{\hat{1}}_j-\hat{Z}_j) \qty(\mathds{\hat{1}}_{j,j+1}+\hat{Z}_{j,j+1}), \\
\hat{L}_{3_{j,j+1}} &=\frac{1}{8}\qty(\mathds{\hat{1}}_j+\hat{Z}_j) \qty(\mathds{\hat{1}}_{j,j+1}-\hat{Z}_{j,j+1}) - \frac{1}{2}\hat{S}^+_j \hat{S}^-_{j+1} - \frac{1}{2}\hat{S}^-_j \hat{S}^+_{j+1} 
+ \frac{1}{8}\qty(\mathds{\hat{1}}_j-\hat{Z}_j) \qty(\mathds{\hat{1}}_{j,j+1}+\hat{Z}_{j,j+1}), \\
\hat{L}_{4_{j,j+1}}  &=\frac{1}{4}\qty(\mathds{\hat{1}}_j-\hat{Z}_j) \qty(\mathds{\hat{1}}_{j,j+1}-\hat{Z}_{j,j+1}) ,
\end{split}
\ea
where $\dyad{0}=\frac{1}{2}\qty(\mathds{\hat{1}}+\hat{Z})$, $\dyad{1}=\frac{1}{2}\qty(\mathds{\hat{1}}-\hat{Z})$, and $\sum_{k=1}^{4} \hat{L}_k=2\,\mathds{\hat{1}}$,
the Lindbladian yields:
\ba
\hat{\mathbb{L}}^\tx{(Dephasing)}=\,&2i\Omega  \sum_{j=1}^N \Big[\big( \hat{S}^+_j \hat{S}^-_{j+1}  + \hat{S}^-_j \hat{S}^+_{j+1} \otimes \mathds{\hat{1}}_j \big) - \big( \mathds{\hat{1}}_j  \otimes \hat{S}^+_j \hat{S}^-_{j+1}  + \hat{S}^-_j \hat{S}^+_{j+1} \big)\Big] \nn\\& -\frac{3N}{4}\qty(\mathds{\hat{1}}\otimes\mathds{\hat{1}}) + \frac{1}{8}\sum_{j=1}^{N} \Big[2\big( \hat{Z}_{j} \hat{Z}_{j+1} \otimes \hat{Z}_{j}\hat{Z}_{j+1} +\hat{Z}_{j} \mathds{\hat{1}}_{j+1} \otimes \hat{Z}_{j}\mathds{\hat{1}}_{j+1} \big) 
\nn\\& \qquad\qquad\qquad\qquad \quad
 +  \mathds{\hat{1}}_{j} \hat{Z}_{j+1} \otimes \hat{Z}_{j} \mathds{\hat{1}}_{j+1} +
\hat{Z}_{j}\mathds{\hat{1}}_{j+1} \otimes  \mathds{\hat{1}}_{j} \hat{Z}_{j+1} \nn\\ &\qquad\qquad\qquad\qquad \quad+ 4 \big( \hat{S}^+_{j} \hat{S}^-_{j+1} \otimes \hat{S}^+_{j} \hat{S}^-_{j+1} +  \hat{S}^+_{j} \hat{S}^-_{j+1} \otimes \hat{S}^-_{j} \hat{S}^+_{j+1} \nn\\ &\qquad\qquad\qquad\qquad\qquad \quad+ \hat{S}^-_{j}\hat{S}^+_{j+1} \otimes \hat{S}^+_{j} \hat{S}^-_{j+1} + \hat{S}^-_{j}\hat{S}^+_{j+1} \otimes \hat{S}^-_{j} \hat{S}^+_{j+1} ) \Big].  
\ea

\section{First excited states of the Dephasing Lindbladian}
There are several degenerate first excited states, depending on the system size $N$.
For $N=3$, these are two first excited states associated with a spectral gap of $\Delta\lambda(N=3)=-1$:
\bs
\ba
    \tilde\rho_5 &= \frac{1}{3}(\dyad{011}{100} + \dyad{101}{010} + \dyad{110}{001})  \\
    \tilde\rho_6 &= 
    \frac{1}{3}(\dyad{001}{110} + \dyad{010}{101})+\dyad{100}{011})
\ea\es
Note that the associated eigenstates correspond to non-physical, non-trace-preserving set of states (that are therefore marked with tilde sign).

For $N=4$, there are \textbf{eight} degenerate eigenstates corresponding to an energy gap of $\Delta\lambda(N=4)=-1$.

For $N=5$, there are \textbf{eight} degenerate eigenstates corresponding to an energy gap of about $\Delta\lambda(N=5)=-0.691$.

For $N=6$, there are \textbf{ten} degenerate eigenstates corresponding to an energy gap of $\Delta\lambda(N=6)=-0.5$.
